# Supplementary material for: Knowledge Graph Enhanced Generative Multi-modal Models for Class-Incremental Learning
Source: arXiv:2503.18403 source file (2025-03-24)
Supplement: Supplementary file 1 [file 5_supp.tex]

\clearpage
\setcounter{page}{1}
\setcounter{section}{0}
\maketitlesupplementary

\begin{figure*}[]
    \centering
    \includegraphics[width=0.93\textwidth]
    {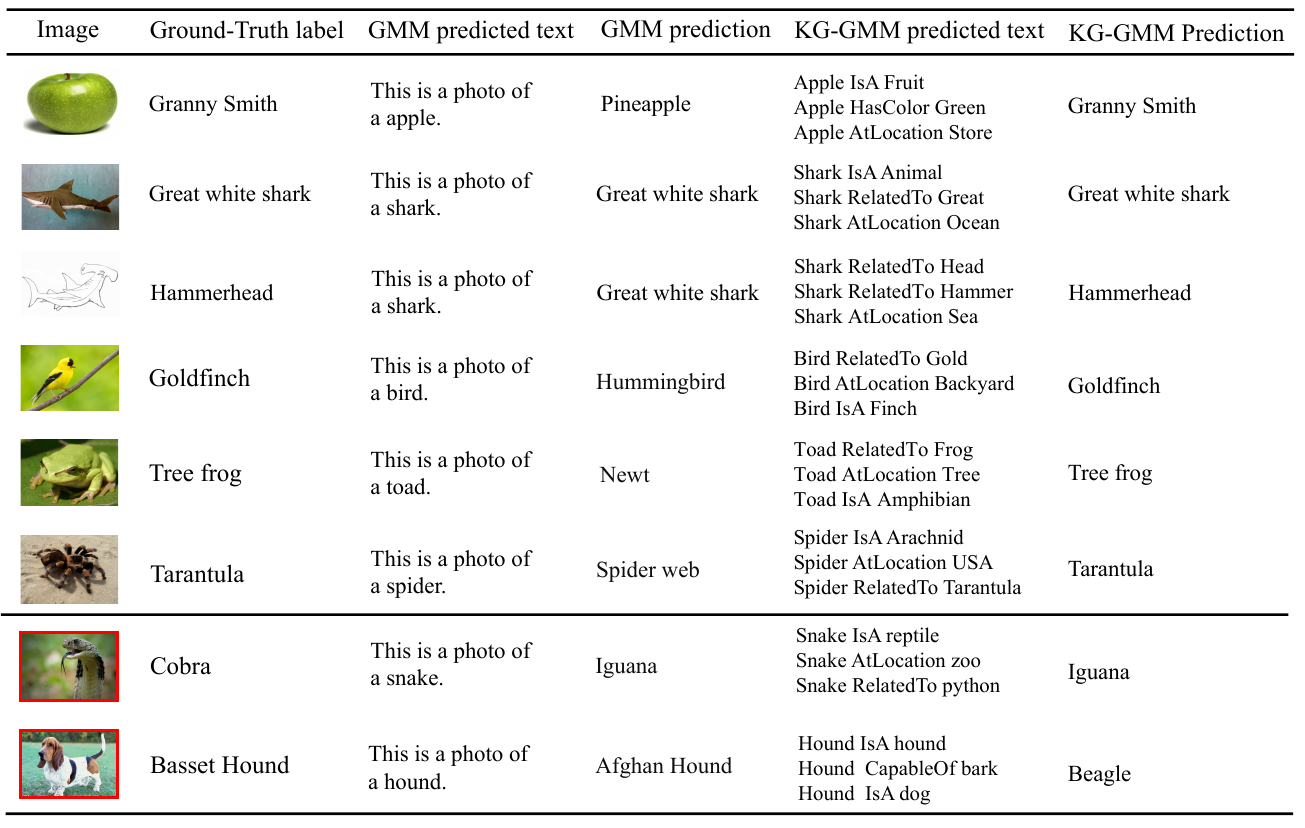}
   
    \caption{More text examples of our methods against the original GMM. The first four examples illustrate how our method corrects the model drift in continual learning. The last two examples with red boxes, showcase where both our method and GMM made incorrect predictions.
    }
    \label{fig_cifar_res}
    \end{figure*}

% \begin{table}

% \caption{Evaluation on B0-10 ImageNet-R with added metrics.}
% \centering
% \vspace{-2pt}
% \label{tab:cifar_few}
% \resizebox{0.45\textwidth}{!}{%   
% \begin{tabular}{c|c|c|c|c}
% \toprule
% Method & Backbone & Last & HAcc($\uparrow$) & Forgetting($\downarrow$)  \\ \midrule
% %ASP  & ViT-B/16         &     &            &           \\
% GMM  & EVA-ViT-G/14          & 80.72    & 79.45           & 8.12          \\
% GMM + EWC  &  EVA-ViT-G/14      & 80.98    & 79.23           & 8.08          \\
% GMM + LwF    &  EVA-ViT-G/14        & 80.82  & 76.33                & 7.95     \\
%  \midrule
% KG-GMM & EVA-ViT-G/14         & 83.60     &   82.50         & 7.54   
% \\ \bottomrule
% \end{tabular}%
% }
% %\vspace{-15pt}
% \label{tab:re}
% \end{table}

\begin{table*}[h]
 \caption{Comparison results between our method and other methods on Tiny-ImageNet and ImageNet-R under different class orders.}
    \centering
    \resizebox{0.95\textwidth}{!}{%
    \begin{tabular}{llcccccccc}
    \toprule
    \multirow{3}{*}{Type}                                                       & \multirow{3}{*}{Method}       & \multirow{3}{*}{\begin{tabular}[c]{@{}c@{}}Exemplar\end{tabular}} & \multicolumn{6}{c}{Tiny-ImageNet}                                                                                                       & ImageNet-R           \\ \cline{4-10}  
                                                                                &                             &                                                                          & \multicolumn{2}{c}{B100-5 tasks}                 & \multicolumn{2}{c}{B100-10 tasks}                & \multicolumn{2}{c}{B100-20 tasks}                & B0-10 tasks             \\
                                                                                &                             &                                                                          & \textbf{Avg}         & \textbf{Last}        & \textbf{Avg}         & \textbf{Last}        & \textbf{Avg}         & \textbf{Last}        & Last                 \\ \hline
    \multirow{7}{*}{Conventional}                                                & EWC~\cite{kirkpatrick2017overcoming}~                        & \XSolidBrush                                                                         & 19.01                & 6.00                 & 15.82                & 3.79                 & 12.35                & 4.73                 & 35.00                 \\
                                                                                & LwF~\cite{li2017learning}          &  \XSolidBrush                                                                        & 22.31                & 7.34                 & 17.34                & 4.73                 & 12.48                & 4.26                 & 38.50                 \\
                                                                                & iCaRL~\cite{rebuffi2017icarl}  & \Checkmark                                                                         & 45.95                & 34.60                & 43.22                & 33.22                & 37.85                & 27.54                & -                    \\
                                                                                & EEIL~\cite{castro2018end}          &  \Checkmark                                                                        & 47.17                & 35.12                & 45.03                & 34.64                & 40.41                & 29.72                & -                    \\
                                                                                & UCIR~\cite{UCIR_2019_CVPR}        &     \Checkmark                                                                     & 50.30                & 39.42                & 48.58                & 37.29                & 42.84                & 30.85                & -                    \\
                                                                                & PASS~\cite{zhu2021prototype}       &   \XSolidBrush                                                                       & 49.54                & 41.64                & 47.19                & 39.27                & 42.01                & 32.93                & -                    \\
                                                                                & DyTox~\cite{douillard2021dytox} & \Checkmark                                                                         & 55.58                & 47.23                & 52.26                & 42.79                & 46.18                & 36.21                & -                    \\ \hline
    \multirow{7}{*}{\begin{tabular}[c]{@{}l@{}}Discriminative \\PT models\end{tabular}}   & Continual-CLIP\cite{thengane2022continualclip}              & \XSolidBrush                                                                         & 70.49       & 66.43      & 70.55     & 66.43       & 70.51       & 66.43       & 72.00                     \\
                                                                                & L2P~\cite{l2p}                         &  \XSolidBrush                                                                         &          83.53            &        78.32              &        76.37              &          65.78            &       68.04               &         52.40             &       72.92                \\
                                                                                % & L2P~\cite{l2p}                         &  \Checkmark                                                                       &        80.24              &     72.89                 &            80.08          &        72.61              &          79.44            &       70.41               &     59.78                \\
                                                                                & DualPrompt~\cite{wang2022dualprompt}                       &  \XSolidBrush                                                                         &      85.15                &    81.01                  &          81.38            &    73.73                  &    73.45                  &      60.16                & 68.82                     \\
                                                                                % & DualPrompt~\cite{wang2022dualprompt}                       &  \Checkmark                                                                        &       79.92               &   72.83                   &      79.15                & 73.21                     &    80.17                  &           71.74           &       57.02               \\
                                                                                 & CODA-Prompt~\cite{smith2023coda}                         & \XSolidBrush                                                                         &             {85.91}         &         {81.36}             &  82.80                    &   75.28                   &          77.43            &  66.32                    &   73.88                   \\
                                                                                & MoE-CLIP~\cite{yu2024boosting}                         & \XSolidBrush                                                                         &  81.12                     &  76.81                     & 80.23                     & 76.35                      & 79.96                      & 75.77                      &  80.87                     \\
                                                                                 & RAPF~\cite{huang2024class}                         & \XSolidBrush                                                                         &  78.64                     & 74.67                      & 77.42                      & 73.57                      & 76.29                      & 72.65                      &  80.28                     \\
                                                                                & Linear Probe                &      \XSolidBrush                                                                     &   74.38                   &          65.40            &         69.73             &     58.31                 &          60.14            &   49.72                   &     45.17                 \\
                                                                                % & Linear Probe                &   \Checkmark                                                                       &    70.10                  &          61.11            &      69.35                &   64.19                   &     71.64                 & 70.50                     &     55.72                 \\ 
                                                                                \hline
    \multirow{6}{*}{\begin{tabular}[c]{@{}l@{}}Generative\\ PT models\end{tabular}} & Zero-shot                   &  \XSolidBrush                                                                         &       58.16               &       53.72               &    58.10                  &           53.72           &           58.13           &         53.72             &       67.38               \\
                                                                                & GMM~\cite{cao2024GMM}                         &  \XSolidBrush                                                                         & 83.42                     & 76.98                     &  82.49                    & 76.51                     & 81.70                     & 76.03                     &        80.72              \\
                                                                                & KG-GMM (Ours) order1                        &  \XSolidBrush                                                                       & 85.88                     & 80.93                   &  {83.91}                   &  {77.35}                    &  {82.98}                   & {77.95}                    &  {84.30}                    \\
                                                                                & KG-GMM (Ours) order2                        &  \XSolidBrush                                                                       & \textbf{86.35}                     & 82.02                   &  {84.45}                   &  {78.47}                    &  \textbf{83.43}                   & \textbf{78.66}                    &  \textbf{84.62}                    \\
                                                                                & KG-GMM (Ours) order3                        &  \XSolidBrush                                                                       & 86.27                     & \textbf{82.62}                   &  \textbf{84.75}                   &  \textbf{78.67}                    &  {83.13}                   & {78.36}                    &  {83.95}                    \\
                                                                                & KG-GMM (Ours)                        &  \XSolidBrush                                                                       & \std{86.17}{0.21}                     & \std{81.86}{0.70}                   &  \std{84.37}{0.35}                   &  \std{78.16}{0.58}                    &  \std{83.18}{0.19}                   & \std{78.32}{0.29}                    &  \std{84.29}{0.27}                   \\
                                                                                % & GMM~\cite{cao2024GMM}                       &  \Checkmark                                                                       & 84.16                     & 78.46                   &  83.95                   &  78.64                    &  84.23                    & 79.17                     &  89.41                    \\
                                                                                  
                                                                                 %  & KG-GMM(Ours)                        &  \Checkmark                                                                       & 85.13                     & 79.55                   &  \textbf{84.62}                   &  \textbf{79.30}                    &  \textbf{84.95}                   & \textbf{80.52}                    &  \textbf{90.14}                    \\
                                                                                
                                                                                %& ours(efficient)             &  0                                                                        &  78.12                    & 69.64                     & 78.60                     &  72.40                    & 77.04                     &  72.47                    &                      \\
                                                                                %& ours(efficient)             &  500                                                                        & \multicolumn{1}{l}{} & \multicolumn{1}{l}{} & \multicolumn{1}{l}{} & \multicolumn{1}{l}{} & \multicolumn{1}{l}{} & \multicolumn{1}{l}{} & \multicolumn{1}{l}{} \\ 
                                                                                \bottomrule
    \end{tabular}%
    }
   
    \label{tab:tiny_CIL_supp}
    
    \end{table*}

\begin{table*}[h]
\caption{Comparison results of our method with other conventional baselines and methods on the mini-ImageNet dataset for few-shot class incremental learning under different class orders. The table includes one base task and eight incremental tasks. \textbf{PD} is the performance drop between the first and last session. $^{*}$ indicates our re-implementation based on PILOT~\cite{sun2023pilot}.}
\centering

\resizebox{0.95\textwidth}{!}{\begin{tblr}{
  hline{1} = {-}{0.08em},
  hline{2, 13} = {-}{},
  hline{19} = {-}{0.08em},
}
            & 0 & 1     & 2     & 3     & 4     & 5     & 6     & 7     & 8     & PD↓ & HAcc↑   \\
iCaRL~\cite{rebuffi2017icarl}       & 61.31   & 46.32 & 42.94 & 37.63 & 30.49 & 24.00    & 20.89 & 18.80  & 17.21 & 44.10 &32.45  \\
EEIL~\cite{castro2018end}        & 61.31   & 46.58 & 44.00    & 37.29 & 33.14 & 27.12 & 24.10  & 21.57 & 19.58 & 41.73 &28.43 \\
LUCIR~\cite{UCIR_2019_CVPR}       & 61.31   & 47.80  & 39.31 & 31.91 & 25.68 & 21.35 & 18.67 & 17.24 & 14.17 & 47.14 &35.65\\
TOPIC~\cite{tao2020few}       & 61.31   & 50.09 & 45.17 & 41.16 & 37.48 & 35.52 & 32.19 & 29.46 & 24.42 & 36.89 &32.98 \\
CEC~\cite{zhang2021few}         & 72.00      & 66.83 & 62.97 & 59.43 & 56.70  & 53.73 & 51.19 & 49.24 & 47.63 & 24.37 &15.96 \\
F2M~\cite{shi2021overcoming}         & 72.05   & 67.47 & 63.16 & 59.70  & 56.71 & 53.77 & 51.11 & 49.21 & 47.84 & 24.21 &19.23 \\
MetaFSCIL~\cite{chi2022metafscil}   & 72.04   & 67.94 & 63.77 & 60.29 & 57.58 & 55.16 & 52.90  & 50.79 & 49.19 & 22.85 &14.35\\
Entropy-reg~\cite{liu2022few} & 71.84   & 67.12 & 63.21 & 59.77 & 57.01 & 53.95 & 51.55 & 49.52 & 48.21 & 23.63 & 19.29\\
L2P$^{*}$~\cite{l2p} & 94.12   &87.20 & 80.99 & 75.67 & 70.94 & 66.76 & 63.11 & 59.81 & 56.83 &  37.29 & 0.0\\
DualPrompt$^{*}$~\cite{wang2022dualprompt} & 93.97   & 86.85 & 80.67 & 75.31 & 70.61 & 66.44 & 62.77 & 59.58 & 56.80 & 37.17 & 0.1  \\
CODA-Prompt$^{*}$~\cite{smith2023coda} & \textbf{95.37}   & 88.86 & 82.69 & 77.87 & 74.47 & 70.16 & 66.46 & 63.73 & 61.14 & 34.23 & 0.0\\
Zero-shot & 58.08   & 58.95 & 57.76 & 57.89 & 58.19 & 57.42 & 56.26 & 54.82 & 54.95 & \textbf{3.13} &52.47 \\
GMM        &  89.35  & 88.40 & 86.11 &85.07  &83.61 & 81.35 & 78.97 & 77.34 & 75.18 & 14.17& 71.45 \\
KG-GMM order1        &  91.32  & {89.87} & {87.92} &{87.67}  &{85.24} & {83.12} & {80.97} & {79.43} & {77.82} & 13.50 & 74.59\\
KG-GMM order2        &  91.54  & \textbf{90.14} & 88.13 &\textbf{87.83}  &85.42 & 83.69 & \textbf{81.45} & \textbf{80.23} & \textbf{78.43} & 13.11 &74.87\\
KG-GMM order3        &  90.12  & 88.40 & \textbf{88.28} &86.37  &\textbf{86.23} & \textbf{84.28} & 80.95 & 79.23 & 77.95 & 12.17 &\textbf{74.96}\\
KG-GMM avg        &  \std{90.99}{0.39}  & \std{89.50}{0.61} & \std{88.11}{0.02} &\std{87.29}{0.43}  &\std{85.63}{0.19} & \std{83.70}{0.22} & \std{81.12}{0.05} & \std{79.63}{0.19} & \std{78.07}{0.07} & \std{12.93}{0.31} &\std{74.81}{0.02}\\
\end{tblr}}

\label{tab:mini_few_supp}
\end{table*}

% \begin{table}

% \caption{Evaluation on B0-10 ImageNet-R with added metrics.}
% \centering
% \vspace{-2pt}
% \label{tab:cifar_few}
% \resizebox{0.45\textwidth}{!}{%
% \begin{tabular}{c|c|c|c|c}
% \toprule
% Method & Backbone & Last & HAcc($\uparrow$) & Forgetting($\downarrow$)  \\ \midrule
% %ASP  & ViT-B/16         &     &            &           \\
% GMM  & EVA-ViT-G/14          & 80.72    & 79.45           & 8.12          \\
% GMM + EWC  &  EVA-ViT-G/14      & 80.98    & 79.23           & 8.08          \\
% GMM + LwF    &  EVA-ViT-G/14        & 80.82  & 76.33                & 7.95     \\
%  \midrule
% KG-GMM & EVA-ViT-G/14         & 83.60     &   82.50         & 7.54   
% \\ \bottomrule
% \end{tabular}%
% }
% %\vspace{-15pt}
% \label{tab:re}
% \end{table}

\section{Different class order}
Since the constructed sub-graph is influenced by the order in which classes are encountered, different class orders result in different sub-graphs. To evaluate this effect, we conducted multiple experiments with varying class sequences, and the results are presented in Tab.~\ref{tab:tiny_CIL_supp} and Tab.~\ref{tab:mini_few_supp}. As shown, while our model’s performance fluctuates due to the order variations, it consistently maintains a high level of accuracy, demonstrating the robustness of our method.
% Here we provide detailed experiments on TinyImageNet, ImageNet-R and mini-ImageNet under different class orders in Tab.~\ref{tab:tiny_CIL_supp} and Tab.~\ref{tab:mini_few_supp}.
%由于我们构造的sub-graph会和见到类的先后顺序相关，不同的class order会构建出不同的sub-graph，所以我们根据不同顺序做了多次实验，结果展示在表1和表2，可以看到我们模型性能确实会由于顺序改变出现波动，但都保持了比较高的水平，展现了我们方法的鲁棒性。
% 我

\section{More visualization results}
In Fig.~\ref{fig_cifar_res}, we provide additional visual examples of our methods against the original GMM.  
It can be observed that KG-GMM utilizes attributes such as the bird’s color and location to refine its classification to the finer-grained category of “goldfinch.” In contrast, the original GMM, although retaining knowledge of the broader category, loses the ability to distinguish finer details after learning additional concepts. However, for certain categories that belong to the same broader class (\eg, hound) and have nearly identical characteristics (i.e., similar relations), our method may still make errors, though it typically misclassifies them into closely related categories (\eg, misclassifying a Basset Hound as a Beagle rather than an Afghan Hound based on text similarity). We believe that if similar classes were more distinctly separated with different relations or finer-grained graphs with detailed attributes were incorporated, it would further enhance our method’s performance.
